# Supplementary material for: POPGym: Benchmarking Partially Observable Reinforcement Learning
Source: arXiv:2303.01859 source file (2023-03-03)
Supplement: Supplementary file 1 [file popgym-public-mean.tex]

\begin{tabular}{lr}
\toprule
 & Mean MMER \\
Model &  \\
\midrule
MLP & -0.010 \\
PosMLP & 0.053 \\
FWP & 0.200 \\
FART & 0.202 \\
S4D & -0.119 \\
TCN & 0.219 \\
Fr.Stack & 0.177 \\
LMU & 0.246 \\
IndRNN & 0.302 \\
Elman & 0.224 \\
GRU & 0.326 \\
LSTM & 0.294 \\
DNC & 0.016 \\
\bottomrule
\end{tabular}
